# Supplementary material for: DRAGON: Drone and Ground Gaussian Splatting for 3D Building Reconstruction
Source: arXiv:2407.01761 source file (2024-07-01)
Supplement: Supplementary file 1 [file tab_supp_eiffel.tex]

% \begin{table*}[h]
% \caption{\textbf{Registration performance comparison.} Eiffel tower}
% \label{table:spsg}
% \centering
% \begin{tabular}{|cc|c|c|c|c|c|}
% \hline
% \multicolumn{2}{|c}{} & \multicolumn{2}{|c}{1-HEADED} & \multicolumn{3}{|c|}{2-HEADED} \\ \cline{3-7}
% \multicolumn{2}{|c}{} & \multicolumn{1}{|c|}{COLMAP} & \multicolumn{1}{c|}{COLMAP} & \multicolumn{1}{c|}{COLMAP} & \multicolumn{1}{c|}{\begin{tabular}[c]{@{}c@{}}DRAGON\\ vanilla\end{tabular}} & \multicolumn{1}{c|}{\begin{tabular}[c]{@{}c@{}}DRAGON\\ DreamSim\end{tabular}} \\ \cline{3-7}
% \multicolumn{2}{|c}{} & \multicolumn{1}{|c|}{drone-only} & \multicolumn{1}{c|}{ground-only} & \multicolumn{3}{c|}{drone\&ground} \\ \hline
% \multicolumn{2}{|c|}{Matched (\%) $\uparrow$}  & 100.00 & 79.58 & 50.00 & 88.00 & \textbf{97.47} \\ \hline
% \multicolumn{1}{|c|}{Errors for matched} & rotation ($^{\circ}$) $\downarrow$ & 0.76/0.68 & 19.13/2.39 & 0.69/0.60 & 0.15/0.12 & \textbf{0.12/0.10} \\ \cline{2-2}
% \multicolumn{1}{|c|}{(Avg/Std)} & position (m) $\downarrow$ & 0.02/0.02 & 0.50/0.05 & 0.02/0.02 & 0.02/0.02 & \textbf{0.01/0.01} \\ \hline
% \end{tabular}
% \end{table*}

\begin{table}[]
\caption{\textbf{Registration performance comparison.} Eiffel tower}
\label{table:spsg-eiffel}
\resizebox{\textwidth}{!}{%
\begin{tabular}{|cc|c|c|}
\hline
\multicolumn{2}{|c|}{}                              & COLMAP & SPSG \\ \hline
\multicolumn{2}{|c|}{Matched (\%) $\uparrow$}       &  50.00   &  50.00  \\ \hline
\multicolumn{1}{|c|}{Errors for matched} & rotation ($^{\circ}$) $\downarrow$ &  0.31/0.08   &  0.53/0.09    \\ \cline{2-4} 
\multicolumn{1}{|c|}{(Avg/Std)}          & position (m) $\downarrow$ &   0.01/0.01     &  0.03/0.02    \\ \hline
\end{tabular}%
}
\end{table}
